# Supplementary material for: Effect of ring stiffness and ambient pressure on the dynamical slowdown in ring polymers
Source: arXiv:2112.02051 source file (2022-03-04)
Supplement: Supplementary file 1 [file Supporting_information.pdf]

# Supplementary Information:
# Effect of ring stiffness and ambient pressure on the dynamical slowdown in ring polymers

Projesh Kumar Roy,[1,2] Pinaki Chaudhuri,[1,2] and Satyavani Vemparala[1,2]

[1] *The Institute of Mathematical Sciences, C.I.T. Campus, Taramani, Chennai 600113, India*
[2] *Homi Bhabha National Institute, Training School Complex, Anushakti Nagar, Mumbai 400094, India*

(Dated: March 4, 2022)

# I. METHODS

## A. Threading-detection using triangulation algorithm

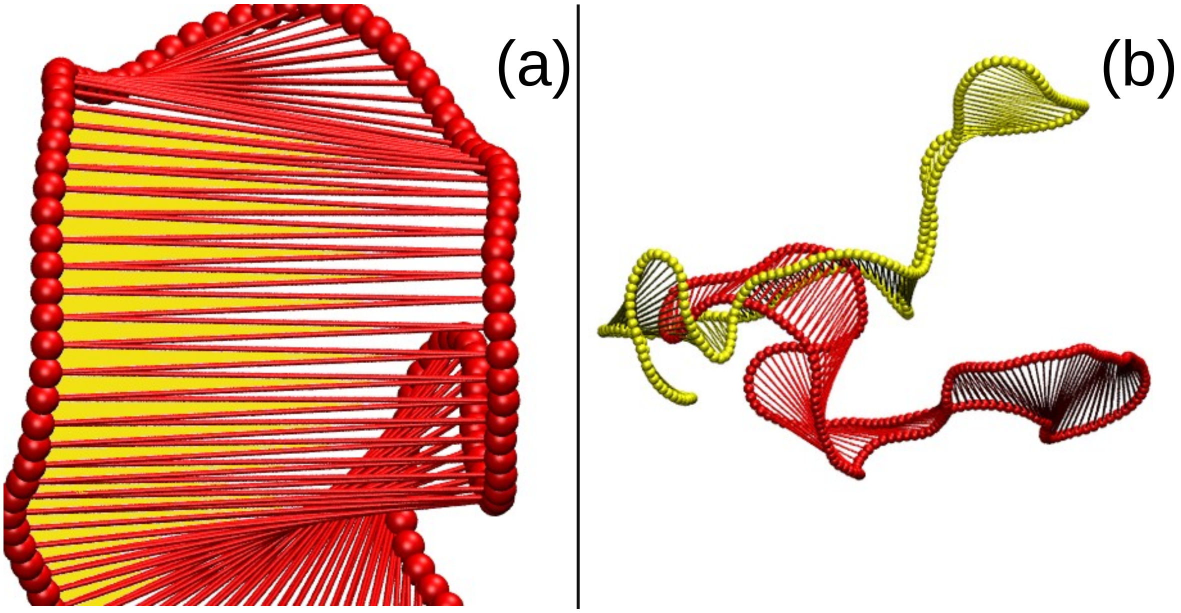


FIG. SI.1: (a): Example of a minimal plane (marked in alternate yellow/white triangles) determined for a crumpled ring-polymer using the triangulation algorithm. (b): Overlap between the minimal surfaces of two ring-polymers.

Identification of the minimal surface, composed of multiple 2D triangles encompassing the 3D structure of the ring polymer [1], is the first part and the key aspect of this algorithm. For this purpose, we use the unwrapped coordinates of the rings, neglecting the periodic boundary conditions. For a perfectly circular structure, the minimal surface of ring-polymer can be easily constructed by drawing criss-cross diagonals using any monomer as the starting point (see Figure SI.1). For irregularly shaped rings, two problems arise. First, one needs to know the monomer corresponding to the starting diagonal. Second, diagonals cannot overlap with each other, otherwise the minimal surface area will be overestimated. The first problem can be solved by directly calculating surface area using all monomers as the starting point and then identifying the monomer corresponding to the minimum surface area. The second problem arises due to loop formation, which allows the diagonals to overlap with each other. This problem requires, i) a decomposition of the deformed polygon into a set of loops, ii) re-calculating the minimal plane for each loop with the previous method, iii) then subsequently joining the loops to create the total minimal surface. We do not consider any self-threading in this algorithm, which further ensures non-crossability of the diagonals. The computational cost for this part is not too large for a 100-mer ring polymer.

The second part of this algorithm is to determine the ring-ring crossing events, by analyzing the overlap between the minimal surfaces of two rings. This part is more time consuming, although efficiency can be increased by using multiple CPU cores and proper parallelization of the algorithm. A further speed-up can be obtained by coarse-graining the ring-polymer geometry [2]. With this method, one can simplify the ring-polymer structure by reducing the number of monomers and thus smoothening the periphery of the ring. The area of the coarse-grained ring is found to be less than the actual ring because of the smoothening. However, the backbone of the coarse-grained ring-polymer remains intact, and can still capture the major threading events. By the term *threading event*, we mean an instance when a bond-vector of one ring polymer passes through the minimal plane of other ring polymer.

## II. RESULTS

### A. Equilibrium dynamics

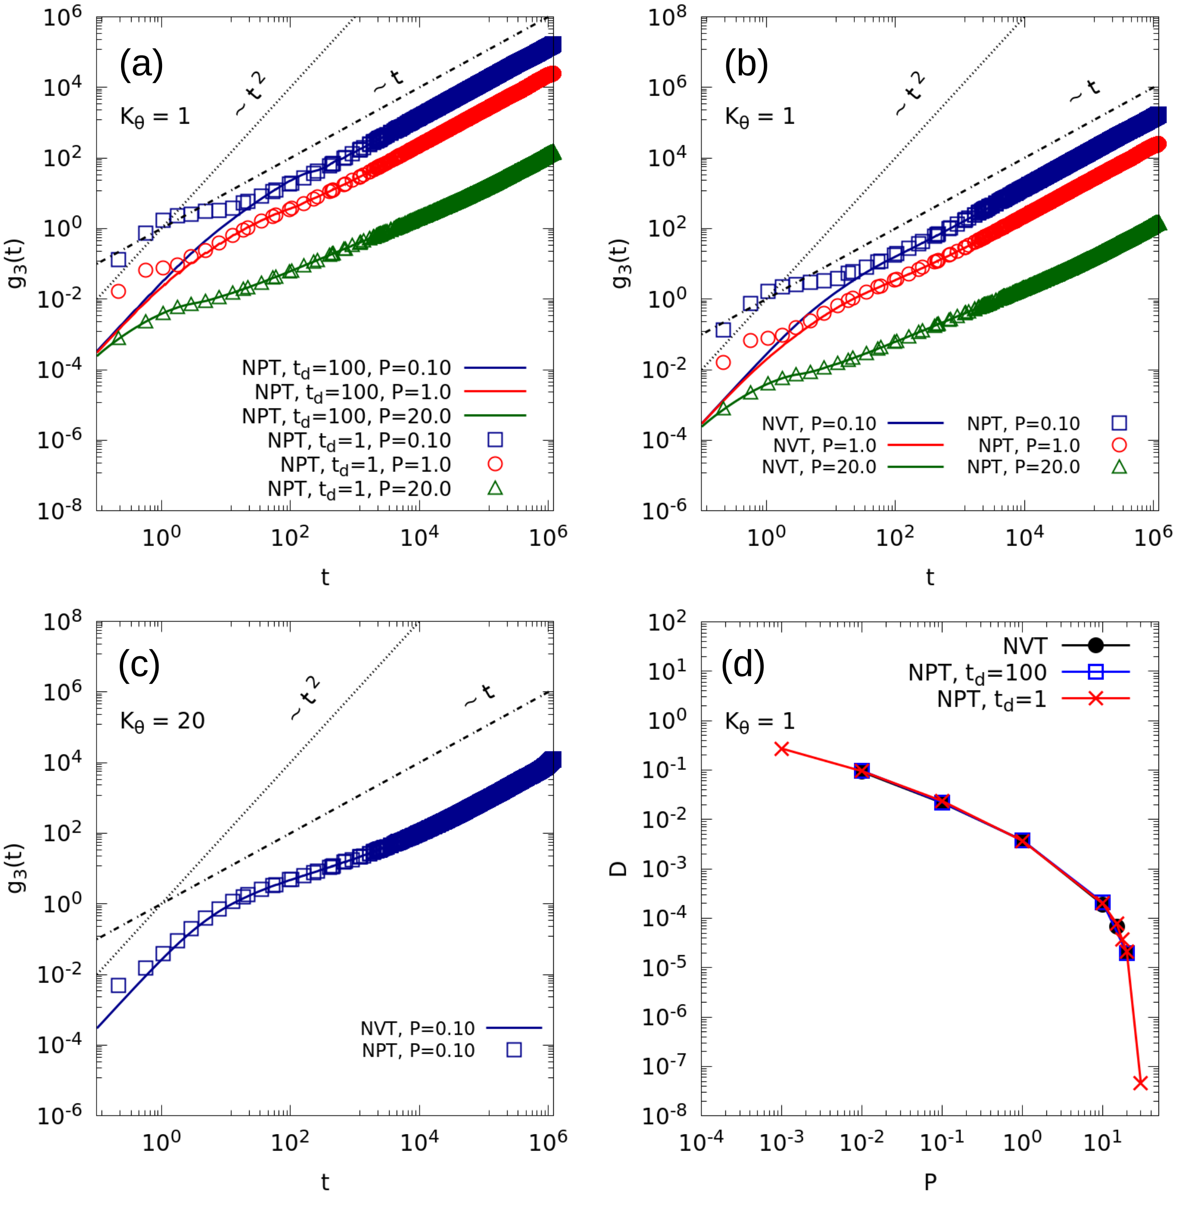


FIG. SI.2: Comparing the behaviour of mean square displacement of the center of the mass of the ring polymers ($g_3(t)$) under different conditions: (a) $t_d$=1 and $t_d$=100 at $K_\theta = 1.0$ for the barostat coupling timescales, (b) NPT (using $t_d$=1) and subsequent NVT simulations at $K_\theta = 1.0$ (with density set to average density obtained for each pressure value under NPT conditions). (c) Similar plot as (b) at $K_\theta = 20$. (d) Comparison of the pressure variation of the diffusion coefficients measured at $K_\theta = 1.0$ from these simulations.

For our study, we have considered the NPT ensemble, i.e. maintaining constant temperature and constant pressure, as is often the situation in experimental conditions. To maintain the desired pressure, we consider a barostat coupling timescale of $t_d = 1$. We have tested that choosing a different $t_d$, e.g. $t_d = 100$, does not affect the long-time diffusive dynamics of the ring polymers at any state point; even though there are variations in the short timescale, which is illustrated in (Figure SI.2(a)). Further, we have also checked that if we use equilibrium states from NPT runs and switch to NVT conditions maintaining the same average density, the long-terms dynamical behavior still remains unchanged, which is expected under equilibrium conditions; see Figure SI.2(b). Consequently, the measured

diffusion coefficients as a function of pressure, remain unchanged regardless of the ensemble used, as is illustrated in Figure SI.2(c).

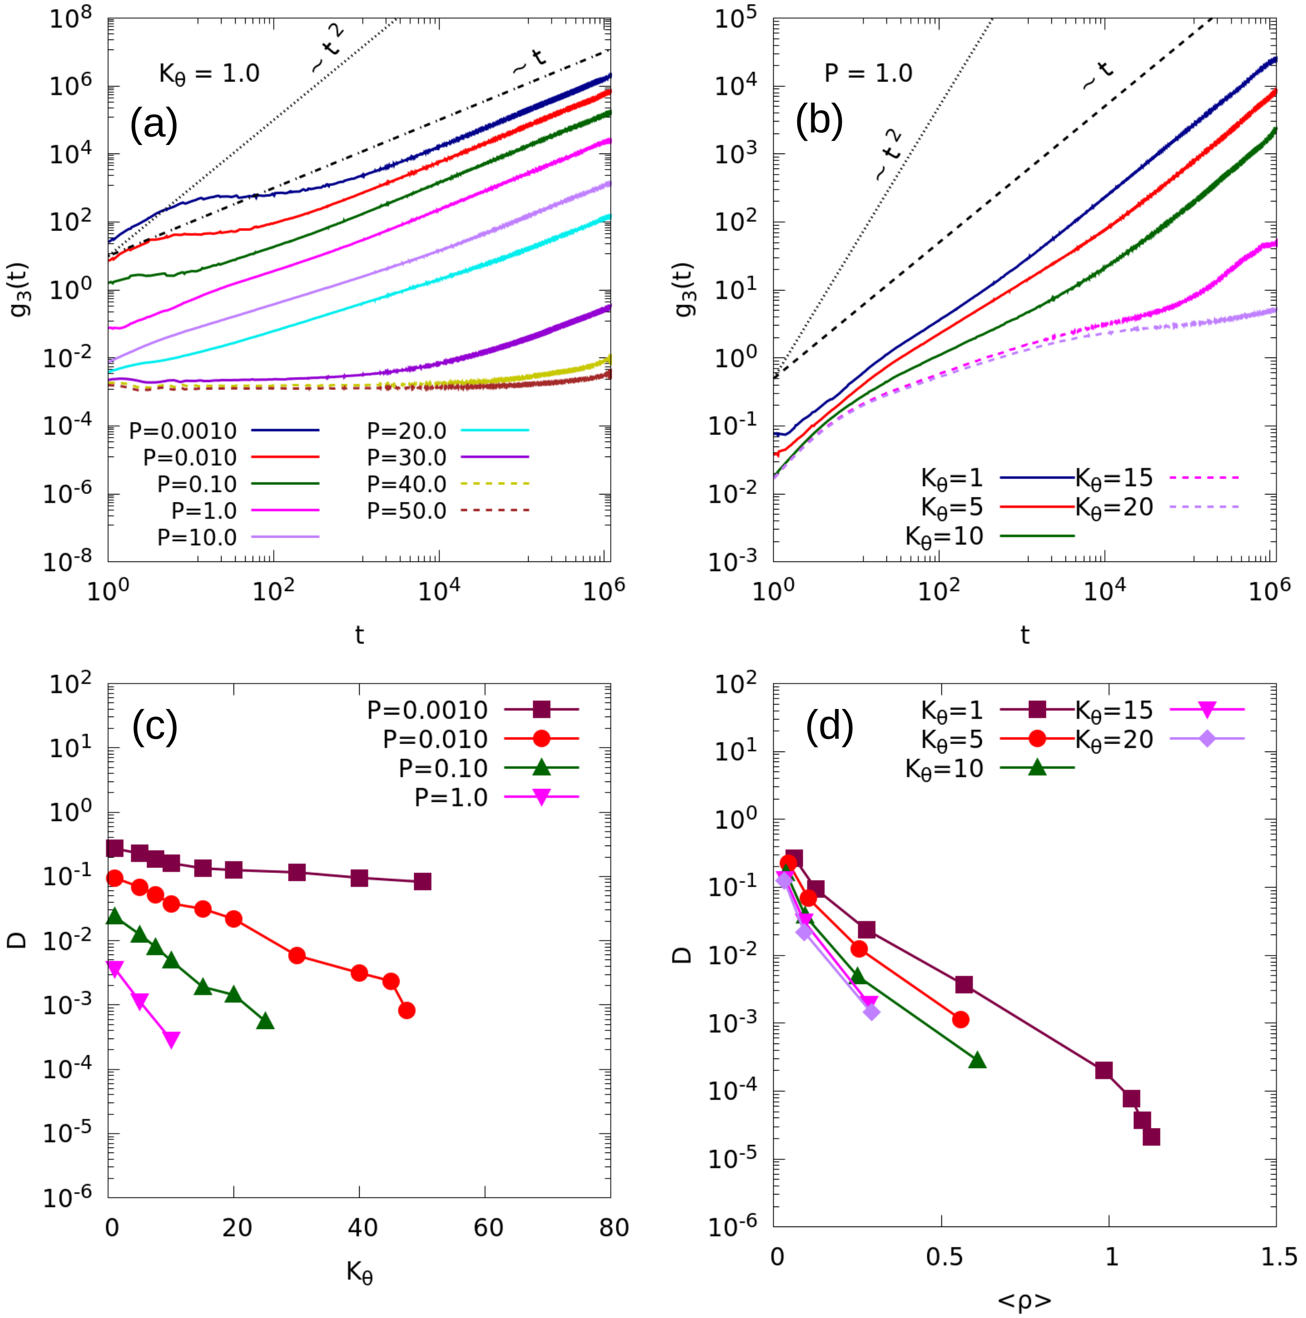


FIG. SI.3: Variation of the mean square deviation of the center-of-masses ($g_3(t)$) of ring-polymers with time at different conditions: (a) at different pressures for $K_\theta = 1.0$, (b) at different $K_\theta$ for P=1.0. Data are shown for regimes where equilibrium has been attained (in solid lines) and where the dynamics is out-of-equilibrium within time-window of observation (in dashed lines). (c) Variation of diffusion constant (D) with various $K_\theta$ values. (d) Variation of diffusion constant (D) at different average densities ($\langle\rho\rangle$).

## B. Structural Characterization

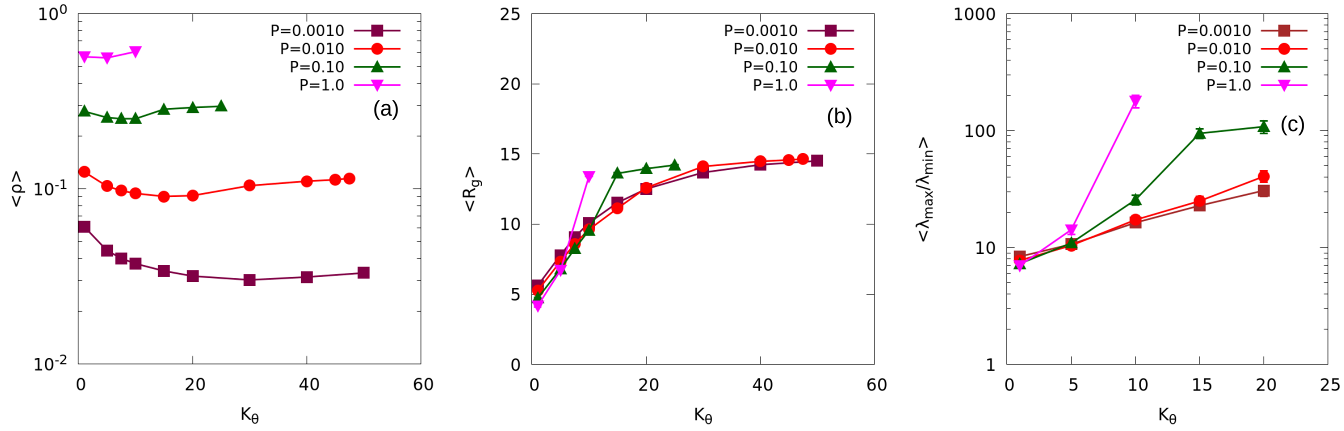


FIG. SI.4: Variation of average density $\langle\rho\rangle$, $\langle R_g\rangle$, and eigenvalue ratio $\langle\lambda_{\max}/\lambda_{\max}\rangle$, for varying stiffness of ring polymers $K_\theta$.

### C. Geometric analysis of the threading events

In this work, we have excluded 5 successive monomers of the ring polymers during coarse-graining the ring periphery. Thus, the effective size of the 100-mer ring polymers is 17 monomers in threading calculations. A center-of-mass cutoff $L_{th} \sim (\sqrt[3]{10^4/\langle\rho\rangle})/2$ is used to identify all possible rings with which a central ring can thread. For the threading correlation function analysis in Figure SI.6 and the corresponding part in the main text, we have used a shorter cutoff $L_{th} \sim 1.5R_g$ upto $t < 1.2 \times 10^3$ and full cutoff beyond that time.

### D. Threading of ring polymers and emergence of spontaneous pinning

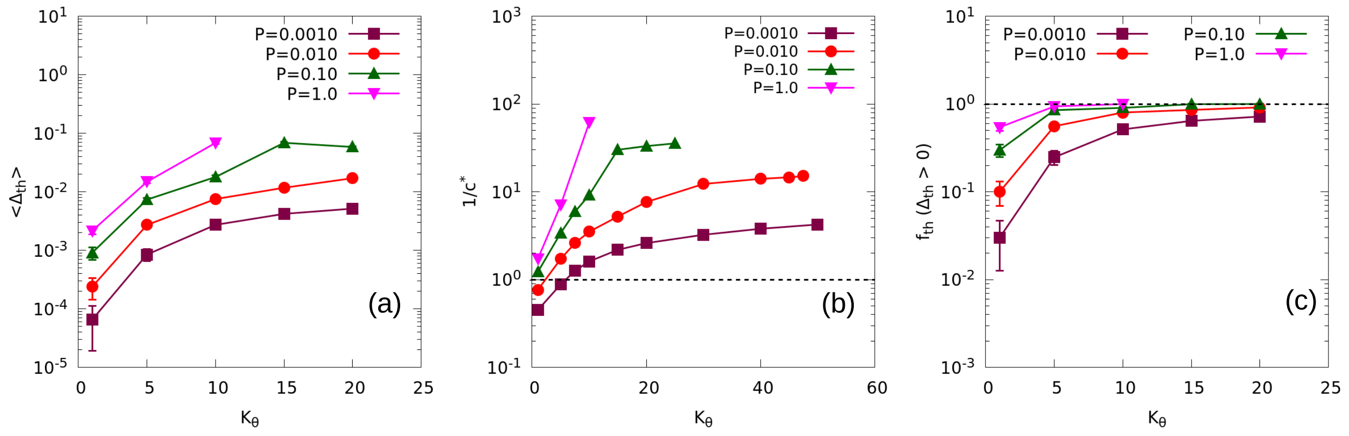


FIG. SI.5: Variation of (a) average threading factor, (b) inverse of the overlap concentration, and (c) average fraction of threaded rings with different $K_\theta$ values. The horizontal dashed line in (b) and (c) cuts the y-axis at 1.

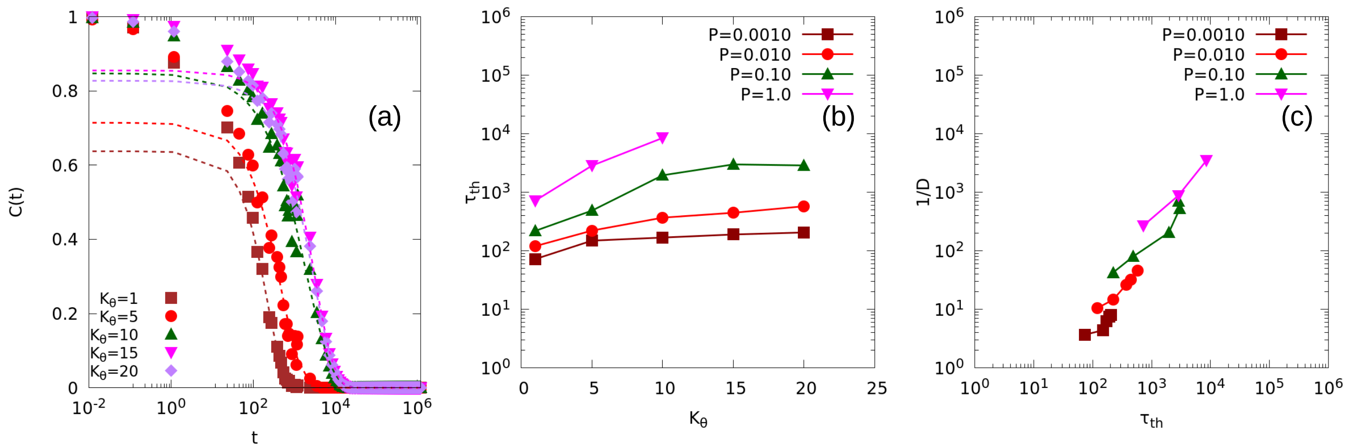


FIG. SI.6: (a) Variation of $C(t)$ with different $K_\theta$ values at P=0.1. A stretched exponential function is used to fit the $C(t)$ data (see main text). (b) Variation of extracted threading timescale, $\tau_{\rm th}$, with $K_\theta$. (c) Correlation plot between inverse of the diffusion coefficient and $\tau_{\rm th}$ for different P-$K_\theta$ state points.

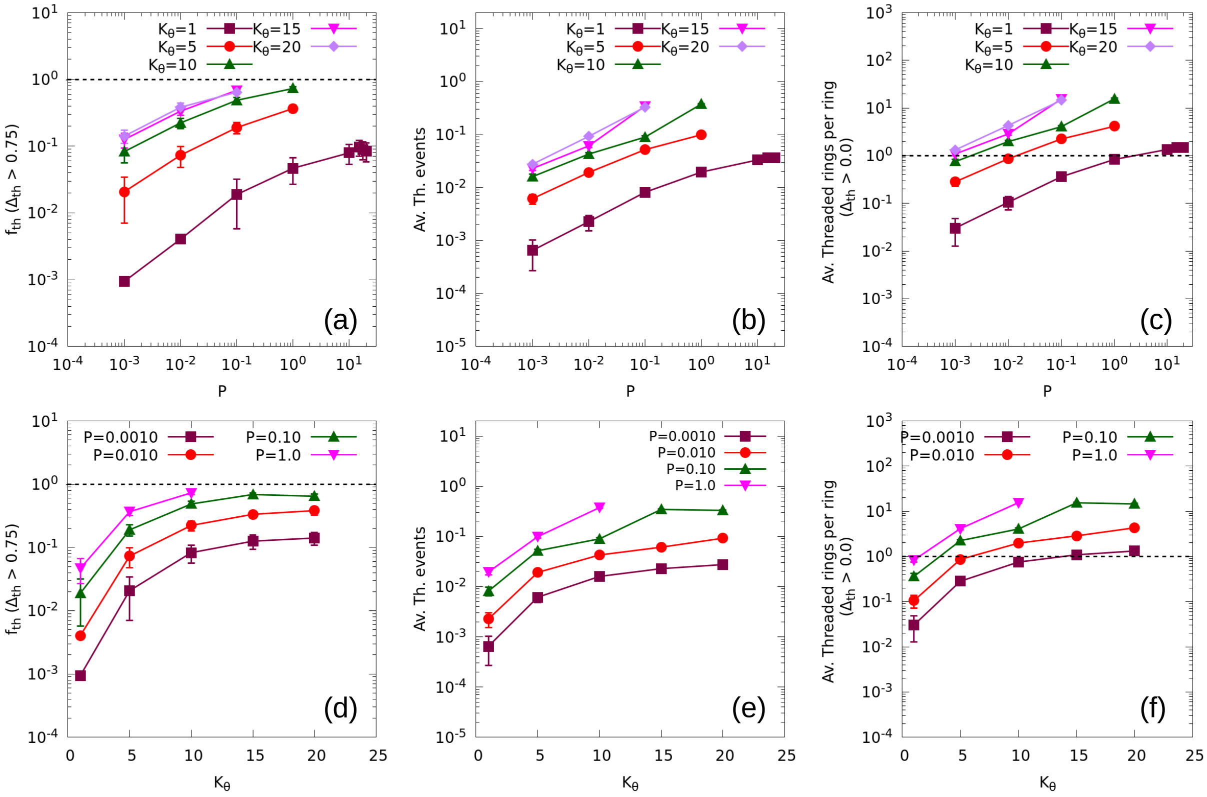


FIG. SI.7: (a)(d) Average fraction of threaded rings with $\Delta_{th} > 0.75$, plotted at different pressure values and $K_\theta$ values, respectively. (b)(e) Average threading events per ring, plotted at different pressure values and $K_\theta$ values, respectively. (c)(f) Average number of rings threaded into one ring, plotted at different pressure values and $K_\theta$ values, respectively. In all figures, the errorbars are included for each data point, except for some data points in $K_\theta$=1, where the errorbar are larger than the data itself. The horizontal dashed line in (a),(c),(d), and (g) cuts the y-axis at 1.

[1] D. G. Tsalikis, V. G. Mavrantzas, and D. Vlassopoulos, Analysis of slow modes in ring polymers: Threading of rings controls long-time relaxation, ACS Macro Letters **5**, 755 (2016), https://doi.org/10.1021/acsmacrolett.6b00259.
[2] F. Guo, K. Li, J. Wu, L. He, and L. Zhang, Effects of topological constraints on penetration structures of semi-flexible ring polymers, Polymers **12**, 2659 (2020).
